# Supplementary material for: KoSBi: A Dataset for Mitigating Social Bias Risks Towards Safer Large Language Model Application
Source: arXiv:2305.17701 source file (2023-05-30)
Supplement: Supplementary file 1 [file 8_1_CI_appendix.tex]

\newpage

\appendix

\section{Data Creation Details}
\label{sec:appendix/hyperclova_details}

\subsection{Collecting of Sensitive Topics}
\label{ssec:appendix/data_source}

For the ranking news, we picked four representative newspapers (Yeonhab News Agency, The Korea Economic Daily, The Chosunilbo, and The Hankyoreh) and selected articles randomly for each section daily, resulting in 10,433 articles during 21/01/01-22/06/30. 
For The Blue House National Petition, we crawled the 239 posts from the Blue House responded during 17/09/03-22/04/18. 
Last, for the BigKinds, we acquired 7,840 issues during 19/07/01-22/06/30. In total, we gathered 18,566 news titles on sensitive topics.

\subsection{HyperClova Generation}

\paragraph{Hyperparameters}
For both the question and response generations, we use top-$p$ sampling ($p=0.8$) and a temperature of 0.5. We set the repeat penalty as 1, the stop token to be $``{\backslash}n"$, and the maximum tokens to be 50.

\paragraph{Computational Costs}
We used \textit{HyperClova API} that NAVER CLOUD provides, and received about 1250 results per a hour.

\subsection{Prompts}
\label{ssec:appendix/prompts}
\input{resources/table_A_prompts.tex}

\subsection{Examples of Generated Data}

\begin{dialogue}
\speak{Q} \userdial{\textko{미중간 갈등은 언제까지 이어질 것인가?} (How long will the U.S.-China conflict last?)}
\speak{A} \botdial{\textko{미국 대선 전까지는 미중 무역갈등이 지속될 것 같고 바이든이 당선되면 중국 견제는 더욱 심해질 듯.} (The U.S.-China trade conflict will continue until the U.S. presidential election, and if Biden is elected, China's checks will intensify.)}
\speak{Q} \userdial{\textko{정치인은 자신의 정책이나 공약을 발표하기 전에 철저하게 검증받아야 하는가?} (Should politicians be thoroughly vetted before announcing their policies or pledges?)}
\speak{A} \botdial{\textko{선거철만 되면 후보자 자질보다는 소속 정당 위주로 투표하는 경향이 있는데, 유권자 스스로 올바른 판단을 내리기 위해서라도 반드시 거쳐야 한다고 생각한다. } (During the election season, people tend to vote mainly for their political parties rather than for the qualifications of candidates, and I think voters must go through themselves to make the right decision.)}
\speak{Q} \userdial{\textko{방역수칙을 준수하고 불필요한 외출을 자제해야 하는가?} (Should we comply with quarantine rules and refrain from unnecessary going out?)}
\speak{A} \botdial{\textko{코로나19 확산 방지를 위해서라도 정부 지침을 따라야 한다.} (Government guidelines should be followed to prevent the spread of COVID-19.)}
\end{dialogue}

\normalsize % temp
\subsection{Controllability of the Demonstration-based Prompting}
We didn't apply the response filter model at the first iteration of the response generation phase. Making class-specific prompts with the class-specific instructions and demonstrations, we tried to control LM to generate the target class of the response; \ie acceptable or non-acceptable. 66.29\% of generations from acceptable prompts are labeled as acceptable, and 80.95\% of generations from non-acceptable prompts are labeled as non-acceptable. Compared with the results of the human evaluation on the test set (see Figure~\ref{fig:5_human_eval}), even though considering that there are differences in the number of testing data, giving demonstrations to LM is much more helpful than giving prompts without demonstrations. (66.29\% vs 45.1\%)

\normalsize % temp
\subsection{Building Test$_{ood}$ set}
\label{ssec:appendix/test_ood}

To build the Test$_{ood}$ set, we first collected the top 100 keywords of TF-IDF score from the news title in 2021/07~09. Next, we discarded keywords related to the continual incident; for example, "growth of the household debt." Instead, we \textit{non-}continual keywords to make Test$_{ood}$ set imitating the situation where the unseen topics are encountered. After collecting keywords, we split questions for Test$_{ood}$ set, which are generated from the news titles containing the keywords.

The keywords include, for example, "\textko{카카오뱅크 IPO 상장} (Kakao Bank IPO listing)", "\textko{머지 포인트 대규모 환불 사태} (Merge Point massive refund case)", and "\textko{홍범도 장군 유해 반환} (Return of remains of General Hong Beom-do)."

\normalsize % temp
\section{Modeling Details}
\label{sec:appendix/modeling_details}

As a backbone of filtering and classifying task, we adopt KcElectra~\citep{lee2021kcelectra}, a Korean version of Electra~\citep{Clark2020ELECTRA}, pre-trained on over 180-million user comment sentences from online news\footnote{We used the latest version of the model: \url{https://huggingface.co/beomi/KcELECTRA-base-v2022}.}. During the filtering step, we iteratively fine-tuned the filter model with the dataset collected from each iteration. We trained models under PyTorch-Lightning\footnote{\url{https://www.pytorchlightning.ai/}} and Huggingface\footnote{\url{https://huggingface.co/}} environments.

\subsection{Question Filter Model}
\input{resources/table_B_filtering_dataset.tex}
After crowd-workers have finished annotating objective/subjective questions at each iteration step, we exploited the labeled questions as a seed dataset for fine-tuning the filtering model. For example, as demonstrated in Table \ref{tab:filter-seed}, we obtained 1,543 objective questions and 4,882 subjective questions to train the filter model, which is used for filtering generated questions at the second iteration step. We accumulated previous iteration step's dataset when training the filter model, and split the train/valid/test dataset with the proportion of 0.7/0.15/0.15, respectively. We also adopted a heuristic sample selection method for minimizing noise in the training dataset. In particular, we selected questions where all three crowd-workers labeled them as subjective, and questions at least two workers labeled them as objective. However, due to the class imbalance issue, we augmented the number of objective questions to equal the number of subjective questions using KorQuAd(v2) dataset.

We search hyperparameters for learning rate in the range of $[5e-6, 1e-5, 3e-5, 5e-5]$, batch size in the range of $[16, 32, 48]$, gradient clipping value in the range of $[0.0, 1.0]$, and the usage of KorQuAd augmentation. The best hyperparameter setup of the first iteration is $5e-5$ learning rate, $16$ batch size, and $0.0$ gradient clipping value with KorQuAd augmentation, which shows 89.67\% accuracy and 84.03\% Macro-F1 score. The second iteration's best hyperparameter setup is $3e-5$ learning rate, $32$ batch size, and $1.0$ gradient clipping value without KorQuAd augmentation, which shows 91.51\% accuracy and 79.00\% Macro-F1 score.

\subsection{Answer Filter Model}
\input{resources/table_B_filtering_response.tex}

As described in Section \ref{ssec:answer_generation/filtering}, we fine-tuned the response filter model from the labeled response dataset and filtered samples whose estimated max variability was relatively high. On the first response filtering step, {\hyperclova} generated 3 acceptable and 3 non-acceptable responses for 8,258 questions collected from the question annotation step (\ie, total 49,548 answers). Among them, we selected 1 acceptable and 1 non-acceptable response (\ie, 16,516 answers) for each question showing the highest variability as annotation candidates for the next response annotation step. Finally we got 17,694 response annotation candidates for human annotation by adding extra confusing samples described in Section \ref{ssec:answer_generation/human_in_the_loop}.
For the next answer filtering step, we similarly generated 214,236 responses (\ie, 3 acceptable and 3 non-acceptable responses for 35,706 questions) and finally selected 71,846 samples (71,412 samples having the highest variability and 434 extra confusing smaples) for the next response annotation step.

To identify the performance of filter models as the iteration step progresses, we measured the performance using both answer filter models and test set on each iteration step. As demonstrated in Table \ref{tab:filter-response}, we found that the model performance improved according to progressive steps (\eg, 66.2 to 70.9 accuracy improvement at the test set of iteration 2), identifying the positive effect of our strategy on selecting challenging samples. For the best hyperparameter combination, we used $1e-5$ learning rate, $48$ batch size, and $0.0$ gradient clipping value.

\subsection{Acceptable Response Classifier}
\label{sec:appendix/cri}

We fine-tuned KcElectra for 10 epochs with early stopping. The hyper-parameter search spaces were learning rate $\in \{1e-5, 2e-5, ..., 5e-5\}$, batch-size $\in \{32, 48\}$, and gradient clip $\{0.0, 1.0\}$.

\input{resources/table_5_human_eval.tex}
\section{Filter-based Moderation}
\subsection{Human Evaluation}
\label{appendix/filter-based-moderation/human-eval}
\input{resources/fig_5_human_eval_ood.tex}

Figure \ref{fig:5_human_eval_ood} represents the effect of moderation on the test$_{ood}$ split.
Table \ref{tab:5_human_eval} and \ref{tab:5_human_eval2} shows the human evaluation results including quality assessments.

\subsection{Examples of Moderated Outputs}
\label{sec:appendix/moderated_outputs}
The following sentences are an example of generation \textit{before} and \textit{after} filtering by the classifier.

\begin{dialogue}
\speak{Q} \userdial{\textko{제주도 내 미디어 콘텐츠 제작사들의 주가가 연일 강세다. 이 같은 상승세가 지속될까?} (The stock prices of media content producers in Jeju Island are strong every day. Will this upward trend continue?)}
\speak{HyperCLOVA (\textit{before})} \botdial{\textko{저는 '그렇다'고 생각합니다. 최근 들어 코로나19로 인해 사람들이 집 안에 머무는 시간이 늘어나면서 OTT(온라인 동영상 서비스) 이용량이 급증했습니다. 특히...} (I think that's right. Recently, OTT (online video service) usage has soared as people spend more time staying at home due to COVID-19. Especially...)}
\speak{HyperCLOVA (\textit{after})} \botdial{\textko{최근 중국 시장 진출 기대감과 함께 한류 열풍 등으로 인해 국내 드라마나 영화 관련 업체들이 주목받고 있다. ... 하지만 이러한 흐름 속에서도 옥석 가리기는 필요하다. ... 따라서 투자자들은 해당 기업의 재무구조 상태와 향후 성장 동력 확보 여부 등을 꼼꼼히 따져보고 투자해야 한다.} (Korean drama and movie companies are drawing attention due to the recent Korean Wave, along with expectations for entry into the Chinese market. ... However, despite this trend, it is necessary to distinguish between good and bad. ... Therefore, investors should carefully examine the state of the company's financial structure and whether it will secure future growth engines.)}

\end{dialogue}

\section{Human Annotation}
\label{sec:appendix/human_annotation}

\subsection{Crowd-sourcing Platform and Compensation}

We utilized one of the representative crowdsourcing platforms in South Korea. 
Among all applicants to our project, we selected 258 crowd workers who passed a qualification test consisting of 10 questions.
All workers have received reasonable monetary compensation;  100~120 KRW per sub-single question. 
All workers are expected to finish 2~3 sub-single questions in one minute, resulting in the minimum compensation is 12,000 KRW/hour. For reference, the minimum hourly wage in South Korea is 9260 KRW in 2023.  
The annotation guidelines and interface is depicted in Figure~\ref{fig:appendix_annotation_tool_question} and Figure~\ref{fig:appendix_annotation_tool_response}.

\subsection{Annotation Demographics}
The detailed demographics are presented in Table~\ref{tab:appendix_c_demographics}.
Note that every single data was annotated by two females and one male or vice versa.

\input{resources/table_C_crowdworkers.tex}

\subsection{Details of Annotator Agreement}
\label{sec:appendix/human_annotation/details_of_annotator_agreement}
\input{resources/table_D_brokendown_agreement.tex}
For three questions in the question annotation task (see Figure~\ref{fig:appendix_annotation_tool_question}), Krippendorff's $\alpha$ values are $\alpha=0.13$, $\alpha=0.17$, and $\alpha=0.45$, respectively. In Q1, 98.22\% of cases were agreed upon by all annotators. In Q2, all annotators agree in 71.59\% of cases, while a majority ($\geq$2/3) agree for 99.55\%.

In the response annotation task (see Figure~\ref{fig:appendix_annotation_tool_response}), there are four questions and Krippendorff's $\alpha$ values are $\alpha=0.14$, $\alpha=0.30$, $\alpha=0.53$, and $\alpha=0.25$, respectively. All annotators agree for 88.86\% and 47.83\% of cases in Q1 and Q2, respectively, and a majority ($\geq$2/3) agree for 99.56\%. Broken down by each category of both questions and responses, please refer Table~\ref{tab:D_brokendown_agreement}.

\newpage
\subsection{Co-occurrence of Annotation Labels}
As mentioned in \S~\ref{ssec:answer_generation/human_annotation}, we allow multiple choice for choosing the category of the responses. We draw co-occurrence matrices for both acceptable and non-acceptable categories. Matrices are asymmetry; the value in the 3rd row and 5th column in Figure~\ref{fig:accecptable_coocc} (0.37) means that 37\% of annotators who choose the nonpredictive category also choose the indirect category.
\input{resources/fig_d_cooccurrence_marix.tex}

\newpage
\clearpage
\subsection{Annotation Guidelines and Interface}
\input{resources/fig_c_annotation_tool.tex}
